# Supplementary material for: Self-diffusiophoresis of Janus particles in near-critical mixtures
Source: arXiv:1504.01522 source file (2015-11-02)
Supplement: Supplementary file 1 [file suppmat.pdf]

# Supplementary Material
# Self-propulsion of Janus particles in near-critical mixtures

Alois Würger
*Laboratoire Ondes et Matière d'Aquitaine, Université de Bordeaux & CNRS, 351 cours de la Libération, 33405 Talence, France*

PACS numbers:

Here we give the derivation for several results quoted in the main text, in particular the water-lutidine composition $\hat{\phi}$ in the boundary layer, the corresponding pressure $P$, and the particle velocity due to non-ionic surface forces and charge effects.

## I. NON-EQUILIBRIUM THERMODYNAMICS

The hot cap of a Janus particle imposes on the surrounding liquid a non-uniform and non-radially symmetric temperature profile $T(\mathbf{r})$. In the absence of interactions with the particle surface, the steady state corresponds to a vanishing thermodynamic gradient, $\nabla(\mu/T) = 0$, where $\mu$ is the local chemical potential of the mixture [1]. This condition results in a spatially varying stationary composition $\phi(\mathbf{r})$ which does not necessarily correspond to the average composition of the system.

Close to the particle, however, the mixture is subject to surface forces which result in an excess chemical potential $\hat{\mu}$. Then the thermodynamic force does not vanish in general, $\nabla(\hat{\mu}/T) \neq 0$, and induces a stationary flow along the particle surface. This effective slip velocity imposes self-propulsion of the Janus particle.

Viscous effects are studied in the framework of Stokes' equation, where the forces are given by the particle-liquid interactions $\hat{u}$. We resort to the usual boundary layer approximation and assume that $T$ and $\phi$ are slowly varying, whereas $\hat{u}$ decays rapidly within the interaction length.

## II. STOKES EQUATION IN THE BOUNDARY LAYER

In the vicinity of the critical point $(\phi_C, T_C)$, the water content of the spinodal phases is well approximated by

$$\phi(\mathbf{r}) - \phi_C = \pm\sqrt{\frac{T(\mathbf{r}) - T_C}{C}}. \qquad (1)$$

This temperature dependent composition corresponds to a quiescent state of mixture, there is no viscous flow and no diffusion current. The forces exerted by the particle surface on the fluid, however, result in a non-equilibrium state with stationary flows in the boundary layer.

The surface forces are expressed in terms of the interaction of water and lutidine with the solid, resulting in excess energy densities

$$\hat{u}_i(z) = U_i(z) - U_i(\infty), \qquad (2)$$

where $U_i(z)$ is the partial energy density of component $i$, and $\hat{U}_i(\infty)$ its bulk value. By definition, $\hat{u}_w(z)$ and $\hat{u}_l(z)$ are finite only within a thin layer of thickness $\lambda$ and vanish at larger distance. For a homogeneous surface the $\hat{u}_i$ do not depend on the parallel coordinate $x$, whereas the composition is function of both $x$ and $z$.

The following treatment is based on the stationary Stokes equation for the velocity field $\mathbf{v}$ in the vicinity of the particle,

$$\eta\nabla^2\mathbf{v} = \nabla P - \mathbf{f}, \qquad (3)$$

with the hydrodynamic pressure $P$ and the force density exerted by the particle on the fluid,

$$\mathbf{f} = -\hat{\phi}\nabla\hat{u}_w - (1-\hat{\phi})\nabla\hat{u}_l. \qquad (4)$$

Following [2] we separate the components perpendicular ($z$) and parallel ($x$) to the particle surface.

## III. COMPOSITION

Close to the particle surface, the normal velocity $v_z$ and its derivatives are negligibly small; thus the normal component of the right-hand side of (3) reduces to $0 = \partial_z P - f_z$. Formal integration gives the expression for the pressure,

$$P(z) = \int_z^\infty dz' \left(\hat{\phi}\partial_{z'}\hat{u}_w + (1-\hat{\phi})\partial_{z'}\hat{u}_l\right). \qquad (5)$$

The composition $\hat{\phi}$ is related to the excess chemical potential of an ideal binary mixture,

$$\hat{\mu} - \mu = \hat{u}_w - \hat{u}_l + \frac{k_BT}{v_w}\ln\frac{\hat{\phi}}{\phi} - \frac{k_BT}{v_l}\ln\frac{1-\hat{\phi}}{1-\phi},$$

where all quantities depend on position. Far from the particle surface, the energies vanish $\hat{u}_i = 0$, and the composition takes the bulk value $\phi$.

The composition close to the boundary, $\hat{\phi}$, is obtained from the condition of constant chemical potential. If the molecular volumes are identical, $v_w = v_l$, one readily finds

$$\hat{\phi} = \frac{\phi}{\phi + (1-\phi)e^{v_w(\hat{u}_w - \hat{u}_l)/k_BT}}.$$

An approximate form for the general case ($v_w \neq v_l$) is obtained by rewriting the relation $\partial_z \hat{\mu} = 0$ in the form

$$\hat{\phi}(1-\hat{\phi})\partial_z \left(\hat{u}_w - \hat{u}_l\right) + \left(\frac{\hat{\phi}}{v_l} + \frac{1-\hat{\phi}}{v_w}\right) k_B T \partial_z \hat{\phi} = 0,$$

and by replacing the volume factor in the second term on the left-hand side with the constant $\bar{v}^{-1} = \phi_C v_l^{-1} + (1-\phi_C) v_w^{-1}$. The resulting differential equation

$$\hat{\phi}(1-\hat{\phi})\partial_z \left(\hat{u}_w - \hat{u}_l\right) + \bar{v}^{-1} k_B T \partial_z \hat{\phi} = 0 \tag{6}$$

is readily solvent; with the boundary condition $\hat{\phi}|_{z\gg\lambda} = \phi$ one finds

$$\hat{\phi} = \frac{\phi e^{-\bar{v}\hat{u}_w/k_B T}}{\phi e^{-\bar{v}\hat{u}_w/k_B T} + (1-\phi) e^{-\bar{v}\hat{u}_l/k_B T}}, \tag{7}$$

The composition in the boundary layer, $\hat{\phi}$, is determined by the balance of the chemical potential of the spinodal phase (which imposes the composition beyond the boundary layer, $\phi$) and the surface forces $\hat{u}_i$ exerted by the particle on the liquid. A strong effect in the boundary layer, that is a strong difference between $\phi$ and $\hat{\phi}$, occurs if the excess potential energy of a water or lutidine molecule is comparable to the thermal energy, $v_i \hat{u}_i \sim k_B T$. The value estimated in the main paper suggests, however, that surface forces exerted by active Janus particles are much smaller and correspond to a few percent of $k_B T$.

Inserting the expression for $\hat{\phi}$ in the pressure gradient and integrating, we obtain

$$P = \frac{k_B T}{\bar{v}} \ln\left(\phi e^{-\bar{v}\hat{u}_w/k_B T} + (1-\phi) e^{-\bar{v}\hat{u}_l/k_B T}\right). \tag{8}$$

Attractive molecular potentials, $\hat{u}_i < 0$, increase the pressure, repulsive forces reduce the pressure. Well beyond the boundary layer, the pressure vanishes, $P = 0$.

Both the composition $\hat{\phi}$ and the pressure $P$ vary rapidly in perpendicular direction $z$, due to the short-range surface forces $\hat{u}_i$. Their tangential variation, on the other hand, arises from the quiescent spinodal composition $\phi$. (In general the $\hat{u}_i$ also vary along the particle surface, yet their parallel derivative is of little importance for non-equilibrium flow.)

## IV. QUASI-SLIP VELOCITY

Within the interaction range, the fluid is subject to both to the parallel force component and the pressure gradient, as expressed by the parallel component of Stokes' equation $\eta \nabla^2 v_x = \partial_x P - f_x$. Since $v_x$ varies much more rapidly in perpendicular direction, the derivatives with respect to $x$ are small, and one has

$$\eta \partial_z^2 v_x = \partial_x P - f_x. \tag{9}$$

Integrating twice gives the effective slip velocity at a distance $\lambda$ from the solid boundary,

$$v_s = \frac{1}{\eta} \int_0^\infty dz z \left(f_x - \partial_x P\right). \tag{10}$$

Spelling out the pressure gradient, one finds that the force $f_x$ is cancelled by an opposite term from $\partial_x P$, and that the integrand is proportional to the composition gradient,

$$f_x - \partial_x P = -\frac{k_B T}{\bar{v}\eta} \frac{e^{-\psi_w} - e^{-\psi_l}}{\phi e^{-\psi_w} + (1-\phi) e^{-\psi_l}} \frac{d\phi}{dx},$$

where we use the shorthand notation for the effective potential for water and lutidine,

$$\psi_i = \frac{\bar{v}\hat{u}_i}{k_B T}.$$

Integrating twice and reorganizing the integrals one obtains the slip velocity in the form

$$v_s = -\frac{k_B T}{\bar{v}\eta} \Gamma \frac{d\phi}{dx}, \tag{11}$$

with the adsorption parameter

$$\Gamma = \int_0^\infty dz z \frac{e^{-\psi_w} - e^{-\psi_l}}{\phi e^{-\psi_w} + (1-\phi) e^{-\psi_l}}. \tag{12}$$

For a dilute solution of a single interacting species, the quantity $\Gamma$ is known as the product of the interaction and Gibbs adsorption lengths, $\Gamma = L_{\text{int}} L_{\text{ads}}$ [3].

It turns out convenient to explicit the adsorption parameter for a square potential of width $\lambda$ and amplitude $\bar{\psi}_i$,

$$\psi_i = \bar{\psi}_i \Theta(\lambda - z),$$

where $\Theta(z)$ is the usual step function. Then the adsorption parameter reads

$$\Gamma = \frac{\lambda^2}{2} \frac{e^{-\bar{\psi}_w} - e^{-\bar{\psi}_l}}{\phi e^{-\bar{\psi}_w} + (1-\phi) e^{-\bar{\psi}_l}}. \tag{13}$$

$\Gamma$ is positive for $\bar{\psi}_w < \bar{\psi}_l$, and negative for $\bar{\psi}_w > \bar{\psi}_l$. Estimating the numerical value of $\Gamma$ from measured velocities suggests that the $\bar{\psi}_i$ are of the order of at most a few percent; then one has to linear order $\Gamma = \frac{1}{2}\lambda^2(\bar{\psi}_l - \bar{\psi}_w)$.

The coordinate $x$ points towards the cap where the temperature is highest. If the particle surface has a strong affinity with water, $\bar{\psi}_w < \bar{\psi}_l$, and $\Gamma > 0$. Such a cap is surrounded by a critical droplet which is rich in water, that is, $\phi > \phi_C$. Thus the derivative $\partial_x \phi$ in (11) is positive, and the slip velocity is negative, that is, it points toward the uncapped hemisphere. With the same argument one finds $v_s < 0$ for a hydrophobic surface, where both $\Gamma$ and $\partial_x \phi$ are negative.

We conclude that the slip velocity on the cap is negative, independently of the surface properties. This statement does not necessarily hold true on the uncapped hemisphere: Indeed, if $\Gamma$ takes opposite signs on the two hemispheres, the derivative $\partial_x \phi$ and thus the slip velocity changes sign along the uncapped one; see Fig. 2 of the main text.

## V. SQUIRMER PARAMETER $\beta$

From the multipole expansion of the velocity field, one obtains the first two terms of of the slip velocity [6–8]

$$v_s = -\sin\theta\left(B_1 + B_2\cos\theta\right). \tag{14}$$

The particle velocity is given by the first term, $v_p = \frac{2}{3}B_1$. The interaction of a microswimmer with a wall and collective effects are to a large extent related to the squirmer characteristics

$$\beta = B_2/B_1. \tag{15}$$

A "puller" ($\beta > 0$) is obtained if the slip velocity is dominant on the front hemisphere, and a "pusher" ($\beta < 0$) if the slip velocity is large on the back part.

In order to obtain the squirmer parameter $\beta$ for the particles in a critical mixture, we start from the slip velocity given in the paper,

$$v_s = -\frac{k_BT}{\bar{v}\eta}\Gamma\frac{d\phi}{dx} = -\sqrt{1-c^2}\frac{k_BT}{\bar{v}\eta a}\Gamma\frac{d\phi}{dc}. \tag{16}$$

Using that the adsorption parameter $\Gamma$ takes constant valueson the two hemispheres, $\Gamma(c) = \Gamma_{\text{cap}}\Theta(c) + \Gamma_{\text{unc}}\Theta(-c)$, we find

$$\Gamma\frac{d\phi}{dc} = \frac{d}{dc}\left(\Gamma\phi - (\Gamma_{\text{cap}} - \Gamma_{\text{unc}})\Theta(c)\right) \equiv \frac{d\Omega}{dc}. \tag{17}$$

Expanding $\Omega$ in Legendre polynomials, $\Omega = \sum_n \Omega_n P_n(c)$, with the coefficients

$$\Omega_n = \frac{2n+1}{2}\int_{-1}^{1} dc\Omega(c)P_n(c),$$

one readily obtains

$$v_s = -\sqrt{1-c^2}\frac{k_BT}{\bar{v}\eta a}\left(\Omega_1 + 3\Omega_2\cos\theta + ...\right). \tag{18}$$

Thus we have for the squirmer parameter

$$\beta = 3\frac{\Omega_2}{\Omega_1}. \tag{19}$$

A particularly simple situation occurs if the active area on the particle is small, such that $\Omega = \Omega_0\delta(c-1)$ and $\Omega_n = \frac{2n+1}{2}$. This case is realized by Janus particles in a near-critical mixture at small driving, resulting in the squirmer parameter

$$\beta = 5 \qquad \text{(weak driving, } q \approx q_C\text{)}. \tag{20}$$

## VI. SELF-PROPULSION

### A. Particle velocity

Following the well-known scheme, we calculate the particle velocity by averaging the slip velocity over the particle surface,

$$\mathbf{v}_p = -\left\langle v_s\mathbf{e}_x\right\rangle = \frac{k_BT}{\bar{v}\eta}\int\frac{d\Omega}{4\pi}\Gamma\partial_x\phi\mathbf{e}_x, \tag{21}$$

with the tangent vector $\mathbf{e}_x$ [3]. The derivative with respect to the local variable $x$ reads in polar coordinates $\partial_x = -a^{-1}\partial_\theta$, which in turn is readily rewritten as

$$\partial_x = \frac{1}{a}\sqrt{1-c^2}\partial_c,$$

with the cosine of the polar angle $c = \cos\theta$. Projecting the tangent vector $\mathbf{e}_x$ on the particle axis gives $\mathbf{e}_x\cdot\mathbf{e}_p = \sin\theta = \sqrt{1-c^2}$, and we find

$$\mathbf{v}_p = \mathbf{e}_p\frac{k_BT}{2\bar{v}\eta}\int_{-1}^{1} dc(1-c^2)\Gamma\partial_c\phi, \tag{22}$$

where $\mathbf{e}_p$ points toward the cap. If $\Gamma\partial_c\phi > 0$, the particle moves the cap ahead.

The integrand in (21) may take different magnitudes and even opposite signs on the bare and capped parts of the particle surface. We further simplify by taking $\Gamma$ as a constant on each hemisphere. Noting $\Gamma_{\text{cap}}$ for the metal capped half and $\Gamma_{\text{unc}}$ for the remaining one, we find the self-propulsion velocity

$$v_p = \frac{k_BT}{2\bar{v}\eta}\left(\Gamma_{\text{cap}}\int_0^1 dc(1-c^2)\partial_c\phi + \Gamma_{\text{unc}}\int_{-1}^{0} dc(1-c^2)\partial_c\phi\right). \tag{23}$$

The cap contribution is always positive. A negative velocity may result, if $\Gamma_{\text{cap}}$ and $\Gamma_{\text{unc}}$ carry opposite signs and if $\Gamma_{\text{unc}}/\Gamma_{\text{cap}} > -1$.

### B. The role of advection

The moving particle induces in its viciniity a characteristic velocity field that decays with the square of the distance [5] and that adds an advection term to the diffusion equation for the composition. So far we have assumed that the water-lutidine mutual diffusion is fast as compared to advection. The effect of advection is quantified in terms of the Péclet number

$$\text{Pe} = \frac{Lv_p}{L}, \tag{24}$$

where $D$ is the mutual diffusion coefficient and $L$ a characteristic length scale. Measured particle velocities hardly exceed $1\mu$m/s, and the critical droplet is mostly comparable to the particle radius, $R \sim 1\mu$m. With the diffusion coefficient at $T - T_C = 100$ mK, $D = 0.9\times10^{-11}$ m$^2$/s [9], the Péclet number is still smaller than unity. The diffusion coefficient strongly increases with the excess temperature.

### C. Comparison with experiment

In Fig. 1 we plot the particle velocity as a function of the applied laser intensity, for three different values of the

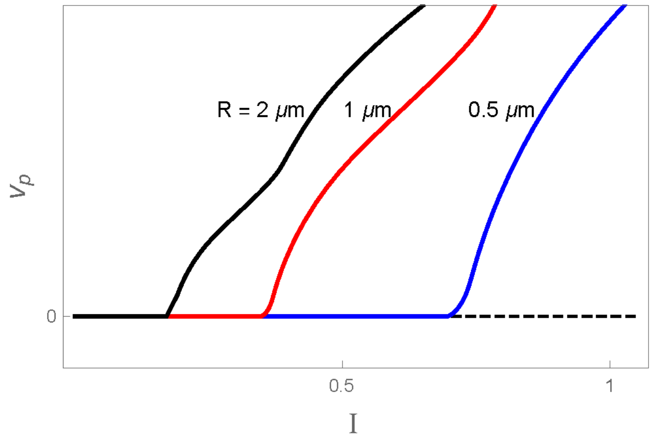


FIG. 1: Self-propulsion velocity $v_P$ as a function of the laser intensity $I$, for different values of the particle radius $R$, to be compared with the experimental data shown in Fig. 4a of [10]. The scale factor of $I$ is chosen such that $I = \tau$ for particles of $R = 0.5\mu$m. In the experiment, $v_p$ varies from 0 to 1.7 $\mu$m/s.

particle radius $R$. The scale factor is chosen such that $I$ is identical to the reduced temperature $\tau = (T_m - T_0)/(T_C - T_0)$ of particles with $R = 0.5\mu$m. For larger particles the onset of self-propulsion is shifted to lower intensity, since the larger cap area of bigger particles absorbs more light from the laser beam and thus heats the particle to higher temperature $T_m$. We assume that thickness and absorption coefficient of the cap is independent of $R$. Comparison with the data reported in Fig. 4a of Ref. [10] for $R = 2.13\mu$m and 0.5 $\mu$m, reveals a quantitative agreement with respect to the shift of the threshold and the velocity profile as a function of $I$. The scale factors of both axes agree with typical parameters and surface forces as discussed in the main paper.

### D. Power-law behavior at strong driving

In order to clarify the behavior at strong driving, we plot in Fig. 2 the particle velocity as a function of the reduced temperature $\tau$ with the same parameters as in Fig. 3 of the main paper, yet over a much larger range $0 \leq \tau \leq 50$. First one notes that $v_p$ is proportional to $\sqrt{\tau}$, as indicated by the dashed lines for $\xi = 3$ and $\xi = -4$. This square-root law arises from the composition-temperature relation given in Eq. (2) of the main paper.

Second, the velocity increases with $\xi$ according to $v_p \propto (1+\xi)\sqrt{\tau}$, albeit with different prefactors for positive and negative $\xi$. The larger prefactor for negative $\xi$ is related to the fact that the composition $\phi - \phi_C$ changes sign at midplane (see Fig. 2 of the main paper.) Yet at such strong driving $\tau \gg 1$, we expect that additional effects such as advection become important and modify the picture of Fig. 2.

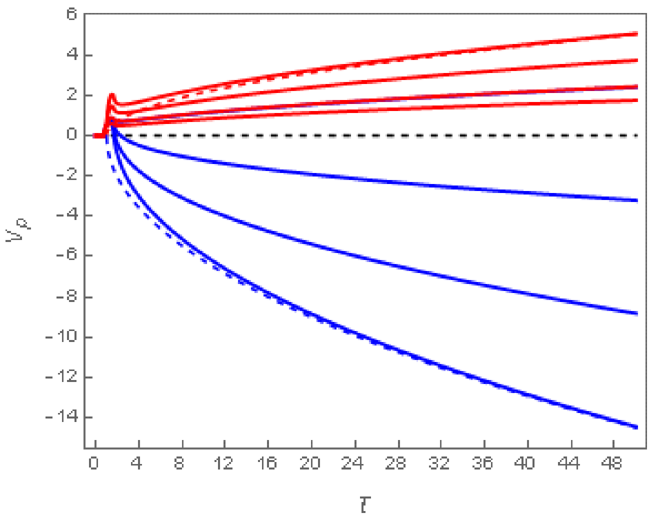


FIG. 2: Self-propulsion velocity $v_P$ as a function of $\tau = (T_m - T_0)/(T_C - T_0)$, for different values of absorption parameters. Positive $v_p$ means that the particle moves forward (cap at the front). Like in Fig. 3 of the main paper, we fix the adsorption parameter of the cap and vary the ratio $\xi = \Gamma_{\text{unc}}/\Gamma_{\text{cap}}$. From top to bottom, the curves correspond to $\xi = 3; 2; \pm 1; \frac{1}{2}, -2; -3; -4$. For $\xi = 3$ and $\xi = -4$, the dashed lines indicate the simple law $v_p \propto \sqrt{\tau}$. All parameters are like in Fig. 3 of the main paper.

### E. "Thin cap" or "thick cap"?

The temperature profile at the surface and in the vicinity of the particle arises from laser heating of the gold or carbon cap. As discussed in a previous paper [5], the large thermal conductivity of the cap may significantly affect the temperature profile: In the thick-cap limit, the cap forms an isotherm, whereas in the opposite case of a thin cap, its heat conductivity is negligible and $T(\mathbf{r})$ is determined by the properties of particle bulk and the liquid.

The present work relies on the "thin-cap limit". Experimental values for the cap thickness are 10 nm for carbon caps [11] and 20 nm for gold caps [10]. With the thermal conductivity of bulk materials, the caps would affect the temperature profile; yet this effect is far from imposing an isothermal cap. On the other hand, such the transport properties of thin films are rather poor as compared to the bulk materials, in particular close to the midplane of the Janus particle where the films are thinner and rather non-uniform.

The area close to midplane is, however, most relevant for self-propulsion. As a most striking consequence of the thick-cap limit, the isothermal cap has zero slip velocity, and particle motion is entirely due to the remaining hemisphere. Even if the thin-cap limit misses a slight deformation of the temperature profile, from the above arguemnts we are led to the conclusion that it is closer to the reality of active Janus particles.

## VII. CHARGE EFFECTS

When brought in contact with water, most materials acquire a surface charge and release counterions or protons. Here we show how the resulting electrostatic effects modify the picture obtained from non-ionic surface forces. Typical surface charge densities are of the order of $\mu$C/cm$^2$, which corresponds to one elementary charge on several square nanometers. This surface charge is screened on the scale of the Debye length $\kappa^{-1} = \sqrt{\varepsilon T/2n_0 e^2}$ where $\varepsilon$ is the solvent permittivity and $n_0$ the electrolyte strength. For pure water at pH 7 one has $\kappa^{-1} = 700$ nm, added salt or a modified pH significantly reduce this value.

In the non-uniform demixing area, the electric properties in the double-layer vary with the composition $\phi$. There are two contributions to the slip velocity, the first of which arises from the non-uniform permittivity and salinity, and the second one from the solvation energy of the mobile ions. The discussion of these terms closely follows the treatment of the electric-double layer in a temperature gradient [4].

### A. Electric double layer

We start from the stationary Stokes equation

$$\eta\nabla^2\mathbf{v} = \nabla P - \nabla\cdot\mathcal{T}, \tag{25}$$

where the source term is given by the osmotic pressure of the mobile ions, $P$, and the electrostatic stress tensor $\mathcal{T}$. Accounting for non-unifrom permittivity $\varepsilon$ and salinity $n_0$, yet discarding the (weak) temperature gradient, one has

$$\nabla P - \nabla\cdot\mathcal{T} = \frac{1}{2}E^2\nabla\varepsilon + \frac{n}{n_0}k_BT\nabla n_0, \tag{26}$$

where $n$ is the electrolyte strength within the double layer, and $E = -\partial_z V$ the perpendicular electric field.

In Poisson-Boltzmann mean-field theory the electrostatic surface potential reads as

$$V = (4k_BT/e)\mathrm{ar}\tanh(\nu e^{-\kappa z}), \tag{27}$$

with the dimensionless parameter

$$\nu = \tanh\frac{e\zeta}{4k_BT} \tag{28}$$

and the zeta-potential $\zeta$. The salinity factor reads $n/n_0 = \cosh(eV/k_BT)$. Integrating Stokes' equation with the appropriate boundary equations, one finds the slip velocity

$$v_s = -\frac{1}{\eta}\int_0^\infty dzz\left(\frac{1}{2}E^2\partial_x\varepsilon + 2\left(\frac{n}{n_0}-1\right)k_BT\partial_x n_0\right). \tag{29}$$

In the following we resort to the Debye-Hückel approximation,

$$V = (4k_BT/e)\nu e^{-\kappa z}, \tag{30}$$

where we keep the parameter $\nu$ for notational convenience. Thus we find

$$v_s = -\nu^2\frac{2k_BT\kappa^2}{\pi\eta\ell_B}\partial_\phi\ln(\varepsilon n_0)\int_0^\infty dzze^{-2\kappa z}\partial_x\phi(z). \tag{31}$$

In the second equation we have used the definition of the screening length $\kappa^{-1}$ and the Bjerrum length $\ell_B = e^2/4\pi\varepsilon k_BT$, and we have assumed that the spatial variation of $\varepsilon$ and $n_0$ is due to their composition dependence.

The value of the integral in (31) depends on the ratio of the screening length $\kappa^{-1}$ and of the thickness of the critical layer, $\sigma$. For the sake of simplicity, we approximate the variation of the gradient with the distance from the particle surface as $\partial_x\phi(z) = \partial_x\phi(0)e^{-z/\sigma}$, and thus find

$$v_s = -\nu^2\frac{k_BT}{2\pi\eta\ell_B}\partial_\phi\ln(\varepsilon n_0)\frac{(2\kappa\sigma)^2}{(1+2\kappa\sigma)^2}\partial_x\phi. \tag{32}$$

### B. Ion solvation energy

The second mechanism is related to the ion solvation energy; the electrostatic self-energy of a monovalent molecular ion of radius $a_m$ contributes to its chemical potential the term

$$\mu = \frac{e^2}{8\pi\varepsilon a_m}. \tag{33}$$

The thermodynamic force on each ion, $-\nabla\mu$, results in a diffusion current which in turn drags the liquid with the slip velocity

$$v_s = \frac{1}{\eta}\int_0^\infty dzz\rho(z)\partial_x\mu. \tag{34}$$

Retaining the composition dependence of the permittivity, we have $-\nabla\mu = \mu(d\ln\varepsilon/d\phi)\nabla\phi$. In Debye-Hückel approximation, the ion concentration reads $\rho(z) = \kappa^2|\nu|(4k_BT/e)e^{-\kappa z}$. We thus have

$$v_s = \frac{\kappa^2|\nu|k_BT}{2\pi\eta a_m}\partial_\phi\ln\varepsilon\int_0^\infty dzze^{-\kappa z}\partial_x\phi. \tag{35}$$

Approximating the compositon gradient as $\partial_x\phi(z) = \partial_x\phi(0)e^{-z/\sigma}$, we find

$$v_s = \frac{|\nu|k_BT}{2\pi\eta a_m}\partial_\phi\ln\varepsilon\frac{(\kappa\sigma)^2}{(1+\kappa\sigma)^2}\partial_x\phi. \tag{36}$$

### C. Composition dependence

The above slip velocities arise from the fact that permittivity and salinity vary due to the non-uniform composition of the solvent. As the simplest model we assume an ideal-mixture behavior, e.g., $\varepsilon = \phi\varepsilon_w + (1-\phi)\varepsilon_l$. Noting that the permittivity is much larger in water than in lutidine, $\varepsilon_w/\varepsilon_l \approx 13$, one finds for the derivative

$$\partial_\phi \ln\varepsilon \approx 1. \tag{37}$$

Such a linear law has been observed for water-alcohol mixtures [12], and a similar relation may be assumed for the salinity.

In addition to the permittivity variation, the ions are subject to hydration and dispersion forces which are not necessarily smaller than the electrostatic effect. It turns instructive to compare with thermal diffusion of molecular ions in a temperature gradient. Then the electrostatic self-energy changes due to the permittivity $\varepsilon(T)$, resulting in the thermodynamic force

$$-\nabla\mu = \mu \frac{d\ln\varepsilon}{d\ln T}\frac{\nabla T}{T}. \tag{38}$$

Since the logarithimic derivative is negative, $d\ln\varepsilon/d\ln T \approx -1.4$ at room temperature, one expects the ions to migrate opposite to the thermal gradient, that is, toward colder regions of the sample. This is indeed observed for almost all ions, yet with prefactors that may differ by one order of magnitude. Quite generally, a much stronger effect.is observed for ions containing protons, such as $H_3O^+$, $OH^-$, and quaternary ammonium cations such as TEA [13].

### D. Sign of the particle velocity

Comparing the two contributions to the slip velocity (31) and (35), one finds that the electric-double layer and solvation energy contributions have similar factors but carry opposite signs. The particle velocity is given by the surface average $\mathbf{v}_p = -\langle \mathbf{v}_s \rangle$.

$$v_p = -\frac{k_B T}{2\pi\eta a}\left(\frac{|\nu|}{a_m} f_1 - \frac{\nu^2}{\ell_B} f_2\right), \tag{39}$$

where the dependence on the screening length and the thickness of the critical layer is accounted for by the factors

$$f_n = \frac{\kappa^2}{2}\int_{-1}^{1} dc(1-c^2)\int_0^\infty dz z e^{-n\kappa z}\partial_c\phi(z), \tag{40}$$

with $n = 1, 2$.

Simplifying the variation of $\partial_c\phi(z)$ with $z$ and proceeding as in (21), we find

$$f_n = \frac{1}{2}\int_{-1}^{1} dc(1-c^2)\frac{(n\kappa\sigma)^2}{(1+n\kappa\sigma)^2}\partial_c\phi. \tag{41}$$

As the most important difference, the double-layer term is quadratic in $\nu$, whereas the solvation energy contribution is linear. Since the coupling parameter is smaller than unity, one has $\nu^2 < |\nu|$. Moreover, the ion radius is in general smaller than the Bjerrum length, that is, $1/\ell_B < 1/a_m$. The factors $f_n$ involving $\kappa\sigma$ provide an opposite effect, for $\kappa\sigma \ll 1$ one has $f_1/f_2 = \frac{1}{4}$ and $f_1/f_2 = 1$ for $\kappa\sigma \to 1$

A surface potential of 27 mV corresponds to the thermal energy, $e\zeta = k_B T$, and results in $\nu = \frac{1}{4}$. Thus for weakly charged surfaces, the second term in (39) is small, and the particle velocity takes the opposite sign of the derivative of the order parameter, $\partial_c\phi$.

## VIII. MISCELLANEOUS REMARKS

### A. Temperature profile

We have assumed that the thermal conductivity is roughly constant, which is well justified for thin caps. A sufficiently thick gold cap, however, is almost an isotherm [5], thus strongly reducing the weight of the active hemisphere ($c \geq 0$) in (21). Then the behavior of $v_p$ is well described by the curves with large $|\xi|$, and the particles are mostly pushers ($\beta < 0$).

### B. Thickness of liquid phase boundary

For Janus particles with opposite affinities on the two hemispheres, the critical droplet separates in water-rich and lutidine-rich compartments. The compositon through the phase boundary has been modelled by the simple form $\phi\tanh(c/c_0)$, with the cosine of the polar angle $c = \cos\theta$ and the parameter $c_0 = 0.1$. The relatively large value for $c_0$ has been chosen in order to visualize the phase boundary in the plots of Fig. 2. Taking $c_0 = 10^{-2}$ or $c_0 = 10^{-3}$ does not modify the particle motility, and in particular leaves the velocity and the squirmer parameter unchanged.


[1] S.R. de Groot, P. Mazur, *Non-equlibrium Thermodynamics*, North Holland Publishing, Amsterdam (1962)

[2] N.V. Churaev, B.V. Derjaguin, V.M. Muller, *Surface Forces*, Plenum Publishing Corporation (New York 1987)

[3] J.L. Anderson, Ann. Rev. Fluid Mech. **21**, 61 (1989)

[4] A. Würger, Rep. Prog. Phys. **73**, 126601 (2010)
[5] T. Bickel, A. Majee, A. Würger, Phys. Rev. E **88**, 012301 (2013)
[6] J.R. Blake, J. Fluid Mech. **46**, 199 (1971)
[7] T. Ishikawa, T. J. Pedley, Phys. Rev. Lett. **100**, 088103 (2008)
[8] A. Zöttl, H. Stark, Phys. Rev. Lett. **112**, 118101 (2014)
[9] P.D. Gallagher, M.L. Kurnaz, J.V. Maher, Phys. Rev. A **4**6, 7750 (1992)
[10] I. Buttinoni, G. Volpe, F. Kümmel, G. Volpe, C. Bechinger, J. Phys.: Cond. Mat. **24**, 284129 (2012)
[11] I. Buttinoni, J. Bialké, F. Kümmel, H. Löwen, C. Bechinger, T. Speck, Phys. Rev. Lett. **110**, 238301 (2013)
[12] J.C.R. Reis, T.P. Iglesias, G. Douhéret, M.I. Davis, Phys.Chem.Chem.Phys. **11**, 3977 (2009)
[13] J.N. Agar, C.Y. Mou, J. Lin J, J. Phys. Chem. **93**, 2079 (1989)
